# Supplementary material for: Single-Photon Structured Light
Source: arXiv:2204.05300 source file (2022-04-11)
Supplement: Supplementary file 1 [file title.tex]

\title{Single-Photon Structured Light\\Supplementary Material}

\author{
  Varun Sundar$\,^{\dagger}$ \quad
  Sizhuo Ma$\,^\dagger$ \quad
  Aswin C.\ Sankaranarayanan$^\ddag$ \quad
  Mohit Gupta$\,^\dagger$ \\
  {$^\dagger$ University of Wisconsin-Madison} \quad
  {$^\ddag$ Carnegie Mellon University}
}
\maketitle
